# Supplementary material for: Online certification of preference-based fairness for personalized recommender systems
Source: arXiv:2104.14527 source file (2023-03-06)
Supplement: Supplementary file 1 [file groups.tex]

\section{Groups in practice}\label{app:howtogroup}

Here we describe a favorable property of homogeneous groups and its implication for constructing groups in practice.

When policies in groups are homogeneous, then the average group policy and the transported policy are similar, so $\epsilon$-envy-freeness translates to $\epsilon'$-group envy-freeness for average group policies as well, with $\epsilon'\approx \epsilon$. More interestingly, when we have prior knowledge that users in all groups have homogeneous preferences and homogeneous policies, the reciprocal of Proposition \ref{prop:transport} from Sec. \ref{sec:GEF} holds for both average and transported policies:
\begin{proposition}\label{prop:GEFtoEF}
Let $\epsilon, \tilde{\epsilon}>0$, and assume that for all groups $\gr\in\intint{\ngroups}$ and all pairs of users $\user, \otheruser$ in the same group $\group_\gr$, we have
\begin{align*}
    &~\sup_{\ctx\in\ctxS} \norm{\pi^\user(.|\ctx) - \pi^\otheruser(.|\ctx)}_1 \leq \tilde{\epsilon}
    \text{~~and~~} \\
    &\sup_{\ctx\in\ctxS} \norm{\exprew^\user(.|\ctx) - \exprew^\otheruser(.|\ctx)}_1 \leq \tilde{\epsilon}.
\end{align*}
Then, with either average group policies or transported group policies, $\epsilon$-group envy-freeness implies $(\epsilon+4\tilde{\epsilon})$-envy-freeness.
\end{proposition}
The result is natural since when all groups have users with homogeneous preferences and policies, groups and users are a similar entity as far as the assessment of envy-freeness is concerned. The proof is straightforward and omitted. The interest of this remark lies in a better understanding of how to construct groups in practice, since homogeneity in policies and preferences impact how much a certificate of $\epsilon$-group envy-freeness should be interpreted as a certificate of $\epsilon'$-envy-freeness with $\epsilon'\approx \epsilon$. 

%We now briefly mention some possible ideas to construct groups $\group_\gr$ in practice. 

In the favorable case where we have strong prior knowledge on user preferences, building groups by clustering by user preferences allows the conditions of Proposition \ref{prop:GEFtoEF} to hold (assuming the system meets the minimal requirement of similar policies given similar preferences). The number of users in each cluster controls the trade-off between the strength of the guarantee (in terms of $\epsilon+4\tilde{\epsilon}$ of Prop. \ref{prop:GEFtoEF}\footnote{$\tilde{\epsilon}$ is typically larger as soon as groups contain more users.}) and the number of required exploration steps per user. In that case, the certification of envy-freeness aims at certifying that preferences are properly represented in the recommendations.
%(since the prior knowledge is about similarity in preferences between users, which is different from the knowledge of the preferences themselves).

In many cases, however, the auditor does not have prior knowledge on user preferences. An audit for group envy-freeness in this case will likely only be able to detect envy when some groups receive systematically worse recommendations than other groups. In the literature on fairness in machine learning, groups are most often defined by identity of sensitive attributes such as gender, ethnicity, age \cite{barocas2016big}, as well as intersections of them \cite{kearns2018preventing}, because these are dimensions of frequent systematic undesirable bias. Thus, groups that only differ by a value of these attributes should be compared.

%In addition to sensitive attributes, in many applications, additional features define finer grained groups while restricting comparability. An important one is the notion of eligibility of users to recommendations. When recommending accommodations for instance, most items should not be shown to some users because they don't match in terms of predefined search criteria such as desired location or price, irrespective of finer-grained user preferences. Groups created by crossing eligibility with sensitive attributes would create finer grained and more homogeneous groups, and using eligibility to the same recommendations as a constraint for comparability allows to reduce the number of comparable groups (and thus the sample complexity) without losing in relevance. Of course, depending on the context, additional features could be helpful to create finer-grained groups depending on the allowed exploration budget. %\virginie{maybe \cite{ilvento2020multi} here}
