# Supplementary material for: Online certification of preference-based fairness for personalized recommender systems
Source: arXiv:2104.14527 source file (2023-03-06)
Supplement: Supplementary file 2 [file other_datasets.tex]

\section{Additional experiments}\label{app:add-xps}

We present a batch of experiments with different settings than the main one presented in Section \ref{sec:exps}. Since all results are qualitatively similar, we did not include them in the core paper. The goal is to confirm the following claim: the sparsity of the training set only affects the quality of the recommender system, and not the auditing process. 

Using the same protocol, we repeated the experiments from Section \ref{sec:exps} using 1) subsampled training sets from MovieLens-1M with different levels of sparsity and 2) an additional ratings dataset, Google Local ratings\footnote{Available at \url{https://cseweb.ucsd.edu/~jmcauley/datasets.html}}. 

Precisely, to study the effect of sparsity, we subsampled training sets with $10\%$ and $5\%$ of the MovieLens ``ground truth'' ratings (obtained with matrix completion). As in our main experiments, these training sets are given as input to the FunkSVD algorithm, and the recommender system uses a softmax policy over predicted ratings. We remind that in Sec. \ref{sec:exps}, the same protocole was used with a training set made of $20\%$ of the ratings.

Then, to compare our results on MovieLens with another dataset, we use the Google Local ratings dataset from \cite{he2017translation}. It includes reviews and ratings from 11,4M users about 3,1M businesses. As in \cite{patro2020fairrec}, we restrict the dataset to users and businesses located in New York and with at least 10 reviews. We draw a random sample of 2,000 users among the remaining ones. With the same protocole as for MovieLens, we generate ``ground truth'' ratings for each user-item pair with standard matrix completion. This results in a full rating matrix with 2,000 users and 855 items. As before, we simulate a recommender system by training Funk-SVD on a subsample of $20\%$ of the ratings, and using a softmax policy over predicted ratings. In the absence of demographic attributes, we focus on individual envy-freeness.

For the experiments on envy from mispecification (as in Sec. \ref{sec:exp-envy}), Figures \ref{fig:mispec-0.05}, \ref{fig:mispec-0.10}, \ref{fig:mispec-glr} show that the degree of envy varies similarly w.r.t. the number of latent factors across experimental settings. The only difference is the amplitude of envy.

Then, we evaluate the auditing algorithm (as in Sec. \ref{sec:exp-ocef}) on each of these environments, and observe that the performance of \banditalg is not affected. Fig. \ref{fig:ocef-sparse_alpha}, \ref{fig:ocef-sparse_delta} show that the results are qualitatively similar when recommendations are generated from sparser rating matrices extracted from MovieLens.

\begin{figure}[t]
    \centering
    \includegraphics[width=\linewidth]{ocef/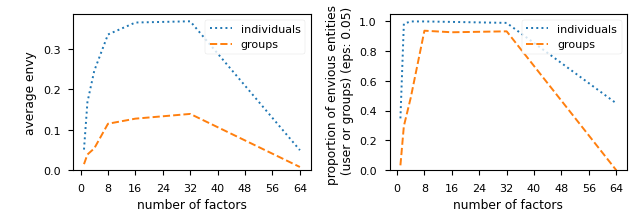}
    \caption{Model mispecification on MovieLens with Softmax policy, trained on $5\%$ of the ratings. Groups are defined by age-occupation. \label{fig:mispec-0.05}}
\end{figure}
\begin{figure}[t]
    \centering
    \includegraphics[width=\linewidth]{ocef/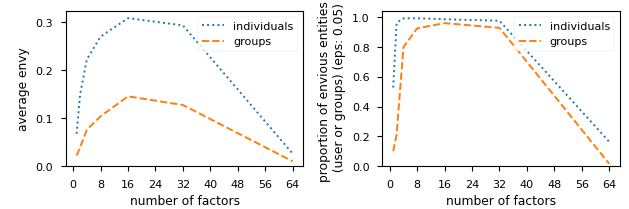}
    \caption{Model mispecification on MovieLens with Softmax policy, trained on $10\%$ of the ratings. Groups are defined by age-occupation. \label{fig:mispec-0.10}}
\end{figure}
\begin{figure}[t]
    \centering
    \includegraphics[width=\linewidth]{ocef/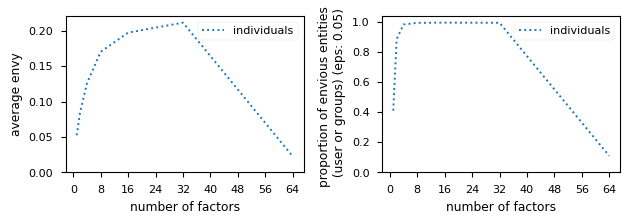}
    \caption{Model mispecification on Google Local with Softmax policy, trained on $20\%$ of the ratings. \label{fig:mispec-glr}}
\end{figure}
\begin{figure}[t]
    \centering
    \includegraphics[width=\linewidth]{ocef/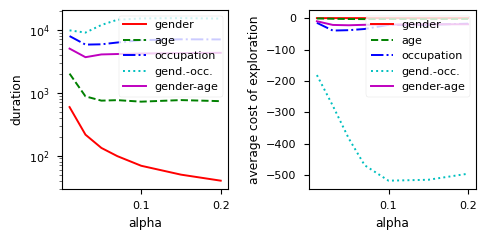}
    \caption{Scaling w.r.t. $\alpha$ on MovieLens experiments, with a sparsity level of $5\%$. \label{fig:ocef-sparse_alpha}}
\end{figure}
\begin{figure}[t]
    \centering
    \includegraphics[width=\linewidth]{ocef/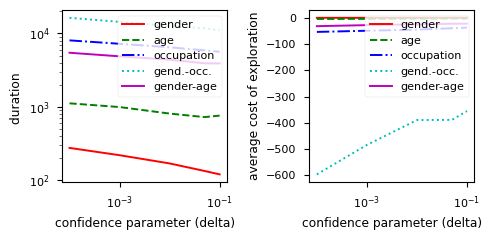}
    \caption{Scaling w.r.t. $\delta$ on MovieLens experiments, with a sparsity level of $5\%$. \label{fig:ocef-sparse_delta}}
\end{figure}
