# Supplementary material for: Online certification of preference-based fairness for personalized recommender systems
Source: arXiv:2104.14527 source file (2023-03-06)
Supplement: Supplementary file 3 [file pull_arm.tex]

\section{The PULL-ARM routine}\label{app:pull-arm}

The PULL-ARM routine used in Alg.~\ref{alg:bandit-sync} is described in Alg.~\ref{alg:pull-sync}.

\begin{algorithm}[t]
\caption{\texttt{PULL-ARM} using transported policies (line 4).\label{alg:pull-sync}}
 \SetKwInOut{Input}{input}\SetKwInOut{Output}{output}
 \SetKwProg{DoParallel}{in parallel}{ do}{end}
 
 \Input{arm $\grarm$, timestep $t$, user group $\group$}
 \Output{Observed group reward $r_t$}
  \ForEach(\tcp*[f]{in parallel}){user $\user \in \group$}{
    Observe context $\ctx^\user_t \sim q^\user$\;
    \lIf{k=0}{$n = m$\tcp*[f]{pull baseline}}
    \lElse{Sample ``other user'' $\otheruser\sim\tilde{\gamma}^*_{m,.}$\tcp*[f]{Def. \ref{dfn:transportedpol}}}
    Show $\act_t^\user \sim \pi^n(.|\ctx^\user_t)$ and observe $\rew^\user_t\sim \nu^\user(\act_t^\user| \ctx^\user_t))$\;
    }
  \Return $\rew_t = \frac{1}{\card{\group}}\sum_{\user\in\group} \rew^\user_t $\;
\end{algorithm}
